# Supplementary material for: A new estimate of mutual information based measure of dependence between two variables: properties and fast implementation
Source: arXiv:1411.2883 source file (2015-09-14)
Supplement: Supplementary file 1 [file supp.pdf]

# Supplementry material for "A new estimate of mutual information based measure of dependence between two variables: properties and fast implementation"

**Namita Jain · C.A. Murthy**

June 12, 2015

## 1 An application to feature selection

An existing dependence measure has been estimated in "Measure of dependence between two variables using mutual information". The resulting estimate called Mutual Information Dependence Index(MIDI) has been used for unsupervised feature selection and results are reported in this section. The usefulness of mutual information for feature selection has been discussed by Liu et al (2009). In this paper we use MIDI to evaluate similarity for feature selection. It may be noted that the maximum value MIDI($d$) can assume is 1. So $1 - d$ is used as a distance between two features. Same, applies to distance correlation and MINE. Pairwise distances between features are calculated and greedy search algorithm is used to select the features. At each step the shortest distance is selected. Among the two features associated with this distance one is selected as given below. The two inputs required are the dataset and number of features to be rejected. The algorithm for feature selection is given below:

1. Calculate the distance between each pair of variables X and Y as $Dist = 1 - d(X, Y)$, where $d(X, Y)$ is the dependence measure calculated using appropriate algorithm (MIDI, dcor or MINE).
2. The values of distance are calculated for each pair of features. Initial sets of selected features and rejected features are null.
3. Sort the values of distance in increasing order.
4. Set $i$ as 1
5. The $i_{th}$ distance from the sorted array is selected.

Namita Jain
Machine Intelligence Unit, Indian Statistical Institute, 203 Barrackpore Trunk Road,Kolkata 700108,India
Tel.: +919874446800
Fax: +91332573357
E-mail: namita.saket@gmail.com

C.A. Murthy
Machine Intelligence Unit, Indian Statistical Institute, 203 Barrackpore Trunk Road,Kolkata 700108,India E-mail: murthy@isical.ac.in

6. If both the features associated with the selected distance are already selected or any of the feature is already rejected goto step 9).
7. If one is selected while other is not yet tested we reject the newly tested feature.
8. If both the features are being tested for the first time we find the sum of distances between the feature under consideration and remaining features. We select the feature for which the calculated sum is greater and reject the other.
9. Increment $i$.
10. Goto step 5) if desired number of features are not yet rejected.

The performance of proposed method is compared with distance correlation defined by SzéKely and Rizzo (2009)and implemented in R Language by SzéKely and Rizzo (2008) and MINE proposed and implemented by Reshef et al (2011) using above procedure for some data sets. The performance is also compared with performance of MICI($\lambda_2$) defined by Mitra et al (2002). The performance of selected feature set has been tested using knn-classifier accuracy. 10-fold cross validation has been done on data sets available at the UCI Machine Learning repository provided by Bache and Lichman (2013), described in table 1. As the performance of knn-classifier depends on number of neighbors considered, the results have been reported for 1NN classifier, 2NN classifier and knn-classifier, where k is given as square root of number of data points in training set. The execution time for algorithms is reported in seconds. Comparison with distance correlation and MINE is done with fewer data sets as execution time for these algorithms is very high. The k-NN classifier accuracy is reported in Tables 2 and 3. For four out of nine data sets proposed method gives better classification accuracy after feature selection. For another four data sets the classification accuracy is same or slightly better as compared to other methods. For one data set the classification accuracy of proposed method is slightly less as compared to performance of MICI.
The time complexity of feature selection using proposed measure is $O(mn\log(n)+m^2n)$, where $m$ is number of dimensions and $n$ is number of points. In terms of execution time proposed method has lowest execution time as compared to all other methods, for all the data sets considered. The execution times for feature selection are reported in tables 4 and 5.

### 1.1 Experimental setup

All the experiments given above have been executed on an Intel Pentium D 925 3.00GHz CPU and 1.5 GB memory. The random numbers have been generated using in-built pseudo-number generators available in R (runif and rnorm). The results being reported are average values for 10 runs.

## 2 Tables

Table 1: Data set used for feature selection

| Dataset | instances | classes | original no. of features | considered no. of features | Remarks |
|---|---|---|---|---|---|
| Iris | 150 | 3 | 4 | 4 | |
| Cancer | 684 | 2 | 9 | 9 | |
| Ionosphere | 351 | 2 | 34 | 34 | |
| Waveform | 5000 | 3 | 21 | 21 | |
| Forest cover | 581012 | 8 | 54 | 10 | 10 numeric attributes |
| Spambase | 4601 | 2 | 57 | 57 | |
| Arrhythmia | 452 | 16 | 279 | 195 | 195 Real valued attributes |
| Mfeat | 2000 | 10 | 649 | 649 | |
| Isolet | 7797 | 26 | 617 | 617 | |

Table 2: Classification accuracy percentage after feature selection for UCI ML datasets, (Columns MINE, Dcor, $\lambda_2$, MIDI show classification accuracy for MINE, distance correlation, MICI and proposed method. $n_R$, $n_D$, $n_{\lambda_2}$, $n_M$ are number of features selected using MINE, distance correlation, MICI and proposed method respectively.)

| Dataset/Algorithm | value of used in knn classifier | MINE | $n_R$ | Dcor | $n_D$ | $\lambda_2$ | $n_{\lambda_2}$ | MIDI | $n_M$ |
|---|---|---|---|---|---|---|---|---|---|
| Iris | $k = \sqrt{\text{no. of training data points}}$ | 96.8 | 2 | 96.8 | 2 | 96.8 | 2 | 96.8 | 2 |
| | $k = 1$ | 95.53 | 2 | 95.33 | 2 | 96.22 | 2 | 95.56 | 2 |
| | $k = 2$ | 96.23 | 2 | 96.23 | 2 | 96.23 | 2 | 96.89 | 2 |
| Cancer | $k = \sqrt{\text{no. of training data points}}$ | 94.73 | 4 | 94.73 | 4 | 95.56 | 4 | 95.75 | 4 |
| | $k = 1$ | 93.73 | 4 | 93.83 | 4 | 93.85 | 4 | 93.85 | 4 |
| | $k = 2$ | 94.3 | 4 | 94.3 | 4 | 94.2 | 4 | 94.3 | 4 |
| Ionosphere | $k = \sqrt{\text{no. of training data points}}$ | 81.34 | 16 | 80.89 | 16 | 82.5 | 16 | 84.6 | 16 |
| | $k = 1$ | 80.34 | 16 | 80.49 | 16 | 85.92 | 16 | 86.89 | 16 |
| | $k = 2$ | 84.34 | 16 | 83.49 | 16 | 86.02 | 16 | 86.6 | 16 |

Table 3: Classification accuracy percentage after feature selection for UCI ML datasets for large datasets, (Columns $\lambda_2$ and MIDI show classification accuracy for MICI and proposed method. $n_{\lambda_2}$, $n_M$ are number of features selected using MICI and proposed method respectively.)

| Dataset/Algorithm | value of used in knn classifier | $\lambda_2$ | $n_{\lambda_2}$ | MIDI | $n_M$ |
|---|---|---|---|---|---|
| Waveform | $k = \sqrt{\text{no. of training data points}}$ | 80.1 | 10 | 83.11 | 10 |
| | $k = 1$ | 73.81 | 10 | 79.87 | 10 |
| | $k = 2$ | 73.92 | 20 | 79.11 | 20 |
| Spambase | $k = \sqrt{\text{no. of training data points}}$ | 79.01 | 29 | 88.02 | 29 |
| | $k = 1$ | 79.01 | 29 | 88.02 | 29 |
| | $k = 2$ | 79.01 | 29 | 88.02 | 29 |
| Forest cover | $k = \sqrt{\text{no. of training data points}}$ | 91.9 | 6 | 92.78 | 6 |
| | $k = 1$ | 94.05 | 6 | 94.08 | 6 |
| | $k = 2$ | 93.83 | 6 | 94.4 | 6 |
| Arrhythmia | $k = \sqrt{\text{no. of training data points}}$ | 93.4 | 100 | 94.09 | 100 |
| | $k = 1$ | 93.1 | 100 | 93.6 | 100 |
| | $k = 2$ | 93.0 | 100 | 93.06 | 100 |
| Mult. Feat | $k = \sqrt{\text{no. of training data points}}$ | 99.34 | 325 | 99.61 | 325 |
| | $k = 1$ | 99.5 | 325 | 99.6 | 325 |
| | $k = 2$ | 99.5 | 325 | 99.6 | 315 |
| Isolet | $k = \sqrt{\text{no. of training data points}}$ | 96.01 | 310 | 99.18 | 310 |
| | $k = 1$ | 95.81 | 310 | 99.17 | 310 |
| | $k = 2$ | 95.79 | 310 | 99.18 | 310 |

Table 4: Run time for Feature selection algorithm for UCI ML small data sets in seconds(Columns MINE, Dcor, $\lambda_2$, MIDI show execution times for feature selection using MINE, distance Correlation, MICI and proposed measure.)

| Dataset/Algorithm | MINE | Dcor | $\lambda_2$ | MIDI |
|---|---|---|---|---|
| Iris | 20.89 | 0.89 | 0.0027 | 0.0023 |
| Cancer | 152.44 | 165.78 | 0.176 | 0.172 |
| Ionosphere | 1217.11 | 171.89 | 0.1496 | 0.1352 |

Table 5: Run time comparison for feature selection in seconds (Columns $\lambda_2$ and MIDI show execution times for feature selection using MICI and proposed measure)

| Dataset/Algorithm | $\lambda_2$ | MIDI |
|---|---|---|
| Waveform | 5.2 | 3.2 |
| Spambase | 4.14 | 2.6 |
| Forest cover | 16 | 14.99 |
| Arrhythmia | 6.95 | 5.1 |
| Mult. Feat | 597 | 140 |
| Isolet | 695.14 | 422.03 |

**References**

Bache K, Lichman M (2013) UCI machine learning repository. URL http://archive.ics.uci.edu/ml

Liu H, Sun J, Liu L, Zhang H (2009) Feature selection with dynamic mutual information. Pattern Recognition 42(7):1330–1339

Mitra P, Murthy CA, Pal SK (2002) Unsupervised feature selection using feature similarity. IEEE Transactions on Pattern Analysis and Machine Intelligence 24(3):301–312

Reshef DN, Reshef YA, Finucane HK, Grossman SR, McVean G, Turnbaugh PJ, Lander ES, Mitzenmacher M, Sabeti PC (2011) Detecting novel associations in large data sets. Science 16:1518–1524

SzéKely GJ, Rizzo ML (2008) Energy: E-statistics (energy statistics). R Foundation for Statistical Computing, Vienna, Austria, URL http://www.R-project.org

SzéKely GJ, Rizzo ML (2009) Brownian distance covariance. Annals of Applied Statistics 3(4):1236–1265
